# Supplementary material for: A View-consistent Sampling Method for Regularized Training of Neural Radiance Fields
Source: arXiv:2507.04408 source file (2025-07-06)
Supplement: Supplementary file 1 [file 6_supplementary.tex]

\section{Approximate Storage Computation}

The storage problem of projection features is addressed by our proposed distillation process as in Sec.~\ref{sec:distillation}, here we show the necessity of it. For a batch of rays with size $|\mathcal{B}|$, the tensor to store the projection features would be of size $|\mathcal{B}| \times M \times N \times C$, where $M$ is the number of sampled points per ray, $N$ is number of input views, and $C$ is the feature dimension. This is prohibitive when the feature dimension $C$ is very large, for example, in 
the common setting where $|\mathcal{B}| = 4096$, $M = 256$, $N = 50$ and $C = 384$, it will consume roughly 80GB memory with float datatype. But if we distill the features such that $C = 32$, the memory requirement becomes roughly 6.7GB.
